# Supplementary material for: Proposal for a micromagnetic standard problem for materials with Dzyaloshinskii-Moriya interaction
Source: arXiv:1803.11174 source file (2018-03-29)
Supplement: Supplementary file 1 [file SupplementaryMaterial.pdf]

# Proposal for a micromagnetic standard problem for materials with Dzyaloshinskii-Moriya interaction - Supplementary Material

David Cortés-Ortuño,[1,*] Marijan Beg,[2] Vanessa Nehruji,[3] Leoni Breth,[1] Ryan Pepper,[1] Thomas Kluyver,[1] Gary Downing,[1] Thorsten Hesjedal,[4] Peter Hatton,[3] Tom Lancaster,[3] Riccardo Hertel,[5] Ondrej Hovorka,[1] and Hans Fangohr[2,1,†]

[1]*Faculty of Engineering and the Environment, University of Southampton, Southampton SO17 1BJ, United Kingdom*

[2]*European XFEL GmbH, Holzkoppel 4, 22869 Schenefeld, Germany*

[3]*Department of Physics, University of Durham, Durham DH1 3LE, United Kingdom*

[4]*Department of Physics, University of Oxford, Oxford OX1 3PU, United Kingdom*

[5]*Université de Strasbourg, CNRS, Institut de Physique et Chimie des Matériaux de Strasbourg, UMR 7504, F-67000 Strasbourg, France*

[*] d.cortes@soton.ac.uk

[†] hans.fangohr@xfel.eu

## S1. THE DZYALOSHINSKII-MORIYA INTERACTION

In the main study we mentioned that the Dzyaloshinskii-Moriya interaction (DMI) is the result of spin orbit (SO) coupling effects. Spin orbit coupling [1] arises from the magnetic interaction between electrons. In an isolated ion, SO coupling induces orbital moments that lead to single-ion anisotropy: a contribution to the energy arising from the direction of the electronic spin $\boldsymbol{S}$ with respect to the system's crystal axes. When ions interact via an exchange interaction in the presence of SO coupling, processes are allowed that combine these interactions. Starting with both ions in their ground states, one such process involves the SO interaction lifting an ion out of its ground state and then the exchange interaction returning it to the ground state. Another involves the exchange interaction lifting an ion from its ground state and then the SO returning it. Taken together, the effect of these processes is to lead to a so-called *anisotropic exchange coupling* which is known as the DMI. [1–4]

The origin of the DMI can be seen following the derivation given by Yosida [1]. We consider the second-order perturbations caused by a perturbation Hamiltonian that includes the separate spin orbit interactions of two ions and the exchange interaction between them:

$$H' = \lambda(\boldsymbol{L}_1 \cdot \boldsymbol{S}_1) + \lambda(\boldsymbol{L}_2 \cdot \boldsymbol{S}_2) + V_{\text{ex}}, \tag{1}$$

where $\lambda$ is a constant and $V_{\text{ex}}$ encodes the exchange coupling. The effective Dzyaloshinskii-Moriya (DM) Hamiltonian is derived by summing the four processes that involve one interaction via the SO and one via the exchange interaction for each ion:

$$H_{\text{DM}} = H_{\text{DM}}^{\text{I}} + H_{\text{DM}}^{\text{II}} + H_{\text{DM}}^{\text{III}} + H_{\text{DM}}^{\text{IV}}. \tag{2}$$

Each contribution is evaluated using the usual procedure for computing second order perturbations, involving the first of the interactions lifting the system from its ground state $|g_1 g_2\rangle$ to a state with one ion excited (that is $|n_1 g_2\rangle$ or $|g_1 n_2\rangle$), and the second returning the system to the ground state. We list the processes below. Process I: Ion 1 lifted from the ground state $g_1$ by the SO interaction and then returned by the exchange interaction between ion 1 in an excited state and ion 2 in the ground state. Following the process by reading from right to left in the usual manner, we have the contribution

$$H_{\rm DM}^{\rm I} = -\lambda \sum_{n_1} \frac{\langle g_1 g_2 | V_{\rm ex} | n_1 g_2 \rangle \langle n_1 | \boldsymbol{L}_1 \cdot \boldsymbol{S}_1 | g_1 \rangle}{E_{n_1} - E_{g_1}}. \tag{3}$$

Process II involves ion 1 being lifted into an excited state by the exchange interaction and then returned by the SO interaction

$$H_{\rm DM}^{\rm II} = -\lambda \sum_{n_1} \frac{\langle g_1 | \boldsymbol{L}_1 \cdot \boldsymbol{S}_1 | n_1 \rangle \langle n_1 g_2 | V_{\rm ex} | g_1 g_2 \rangle}{E_{n_1} - E_{g_1}}. \tag{4}$$

Processes III and IV are analogous to the I and II, with ions 1 and 2 interchanged. Process III is then

$$H_{\rm DM}^{\rm III} = -\lambda \sum_{n_2} \frac{\langle g_1 g_2 | V_{\rm ex} | g_1 n_2 \rangle \langle n_2 | \boldsymbol{L}_2 \cdot \boldsymbol{S}_2 | g_2 \rangle}{E_{n_2} - E_{g_2}}. \tag{5}$$

Finally, process 4 is

$$H_{\rm DM}^{\rm IV} = -\lambda \sum_{n_2} \frac{\langle g_2 | \boldsymbol{L}_2 \cdot \boldsymbol{S}_2 | n_2 \rangle \langle g_1 n_2 | V_{\rm ex} | g_1 g_2 \rangle}{E_{n_2} - E_{g_2}}. \tag{6}$$

We define the exchange constants $J$, for interactions between excited state ions and ground state ions. For the interaction between ion 2 in the ground state and ion 1 in an excited state, for example, this is written

$$\langle n_1 g_2 | V_{\rm ex} | g_1 g_2 \rangle = -2J(n_1, g_2, g_1, g_2) \boldsymbol{S}_1 \cdot \boldsymbol{S}_2. \tag{7}$$

Since we are always dealing with a single ion in an excited state in any process, it is consistent to operate with the $i$th component of the operator $\boldsymbol{S}_j^{(i)}$for ion $j$ on $|n_j\rangle$ in each of the SO terms and extract its eigenvalue. Noting that the expectation value for the orbital angular momentum $\boldsymbol{L}$ is imaginary allows this, and we find the interaction to be

$$H_{\rm DM} = 2\lambda \sum_i \left\{ \sum_{n_1} \frac{J(n_1, g_2, g_1, g_2) \langle g_1 | L_1^{(i)} | n_1 \rangle \left[ S_1^{(i)}, (\boldsymbol{S}_1 \cdot \boldsymbol{S}_2) \right]}{E_{n_1} - E_{g_1}} \right.$$
$$\left. + \sum_{n_2} \frac{J(g_1, n_2, g_1, g_2) \langle g_2 | L_2^{(i)} | n_2 \rangle \left[ S_2^{(i)}, (\boldsymbol{S}_1 \cdot \boldsymbol{S}_2) \right]}{E_{n_2} - E_{g_2}} \right\}. \tag{8}$$

Finally, using the commutation relation $[\boldsymbol{S}_1, (\boldsymbol{S}_1 \cdot \boldsymbol{S}_2)] = -\mathrm{i} \boldsymbol{S}_1 \times \boldsymbol{S}_2$, we then have an effective Hamiltonian

$$H_{\mathrm{DM}} = \boldsymbol{D} \cdot \boldsymbol{S}_1 \times \boldsymbol{S}_2, \tag{9}$$

with DM vector

$$\boldsymbol{D} = -2\mathrm{i}\lambda \left( \sum_{n_1} \frac{J(n_1, g_2, g_1, g_2)\langle g_1|\boldsymbol{L}_1|n_1\rangle}{E_{n_1} - E_{g_1}} + \sum_{n_2} \frac{J(g_1, n_2, g_1, g_2)\langle g_2|\boldsymbol{L}_2|n_2\rangle}{E_{n_2} - E_{g_2}} \right). \tag{10}$$

The orbital operator $\boldsymbol{L}$ in these expressions makes manifest the vector nature of $\boldsymbol{D}$. As mentioned in the main text, $\boldsymbol{D}$, and thus the Hamiltonian given by equation 9, are constrained by the symmetry of the crystal. As a result, if the two ions have a centre of inversion midway between them, such that the symmetry operation swaps $\boldsymbol{S}_1 \leftrightarrow -\boldsymbol{S}_2$, this implies $H_{\mathrm{DM}} = -H_{\mathrm{DM}}$ and so $H_{\mathrm{DM}} = 0$, implying that $\boldsymbol{D}$ must vanish. A slightly less dramatic example involves a mirror plane running perpendicular to the vector separating the ions, passing through its midpoint, as discussed in Section IIsection*.4 of the main study.

For a pair of ions, it is usually possible to strongly constrain the direction of $\boldsymbol{D}$ through symmetry arguments. This is also valid for the continuum version of the DMI. Nevertheless, we mentioned in Section IIsection*.4 that the Lifshitz invariants [5] (LIs) formalism is required in this limit and the DMI energy can be simplified to depend on a single $D$ parameter. Micromagnetic expressions of the DMI are equivalent to the discrete version of the interaction, as can be seen by considering simple examples. For a planar $C_{2v}$ molecule such as $H_2O$, for example, the vector $\boldsymbol{D}$ is constrained by symmetry to point perpendicular to the plane of the molecule [1]. Discretising the continuum expression for $C_{nv}$ symmetry in the text (see equation 8equation.3.8) shows the absence of the spin components that would be proportional to $D_z$ in the discrete version. Taking to account how the spins are separated in space then gives a contribution to the Hamiltonian equivalent to having a single component of $\boldsymbol{D}$ perpendicular to the plane of the molecule, with magnitude $D$.

## S2. ONE-DIMENSIONAL PROBLEM: MuMax3 RESULTS

Since we consider a one dimensional system of 1 nm in width using a single cell along this dimension, one can expect effects on the spins at the boundaries along the $y$-direction when discretising the system with smaller cells (and thus a larger number of them along the width of the wire). In the MuMax3 code, Neumann boundary conditions are explicitly imposed for the DMI calculation [6], hence effects along the width are observed when modeling a single-cell-wide system. This effect can be suppressed by reducing the system width towards zero, since the continuum analytical model is defined without width. However, it must be present that for real systems, the discretisation should not be smaller than the atomistic spacing. In Fig. S1 we show results from MuMax3 simulations when using a a 1-nm-wide single cell. We observe a disagreement when comparing the results with Fidimag simulations and the theoretical model.

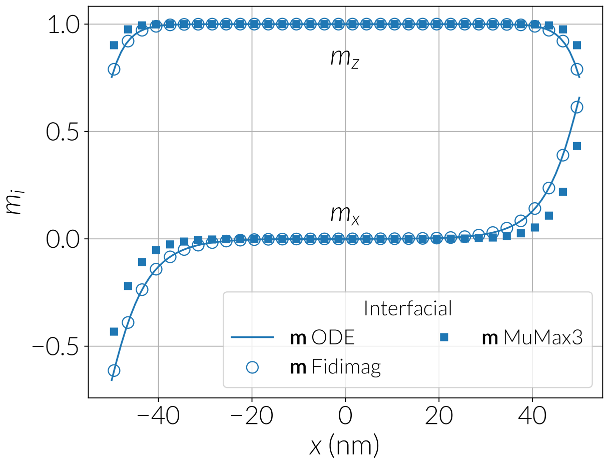


SUPP. FIG. S1. Comparison of the magnetization components along a one-dimensional permalloy-like wire with interfacial DMI. The wire long axis is specified in the $x$-direction. The plot shows solutions from a theoretical description of the system using an ordinary differential equation (ODE) and solutions from simulations using the Fidimag and MuMax3 codes. In this figure the calculations with the MuMax3 code were performed without imposing periodic boundaries along the $y$-direction as in the main study (see Fig. 1Comparison of the magnetization components along a one-dimensional permalloy-like wire with interfacial (a) or bulk (b) DMI. The wire long axis is specified in the $x$-direction. The plot shows solutions from a theoretical description of the system using an ordinary differential equation (ODE), and solutions from the simulations using the OOMMF, Fidimag and MuMax3 codesfigure.1).

## S3. TWO-DIMENSIONAL PROBLEM: CODES COMPARISON

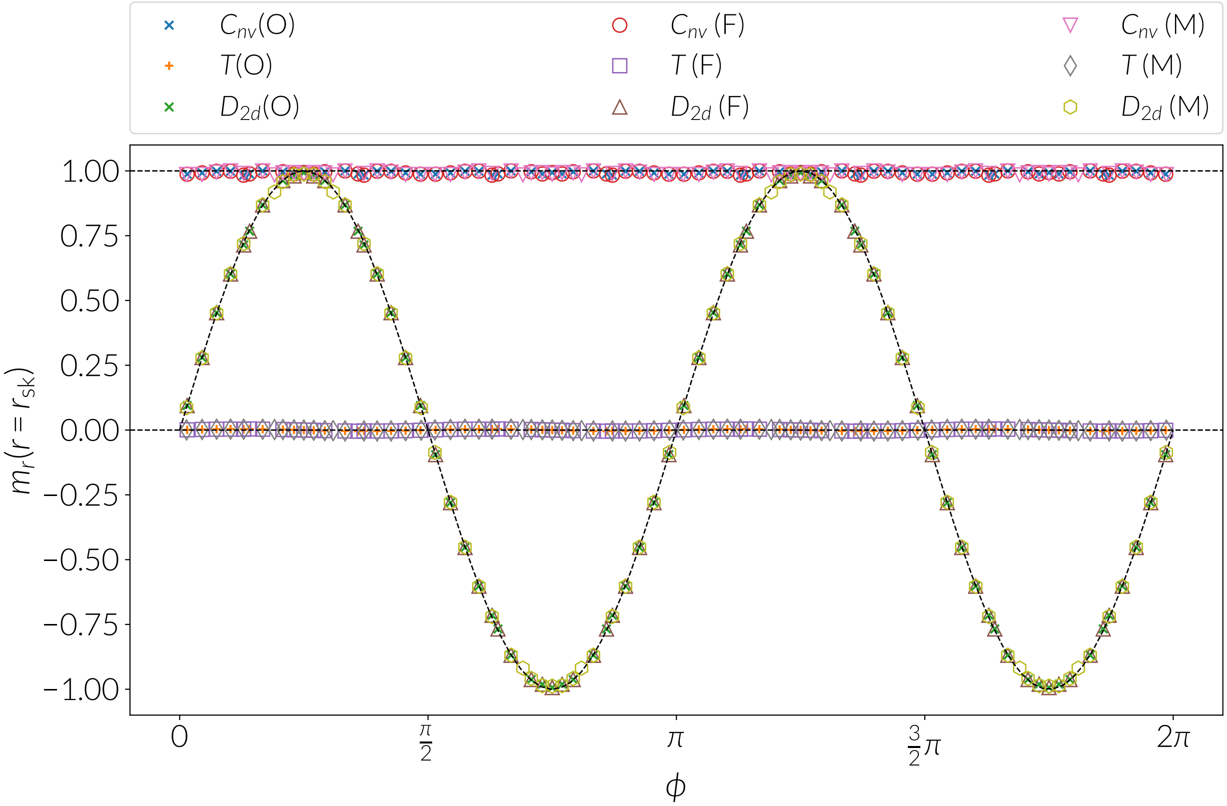


SUPP. FIG. S2. Radial component of the magnetisation at the skyrmion radius, $r = r_{\mathrm{sk}}$, in the disk system defined in the two-dimensional case problem of the main manuscript (Section Vsection*.7), using three different kind of DMI. We show a comparison of the simulation results obtained using Fidimag (F), OOMMF (O) and MuMax3 (M) codes.

## S4. THREE-DIMENSIONAL PROBLEM. COMPARISON WITH THEORY

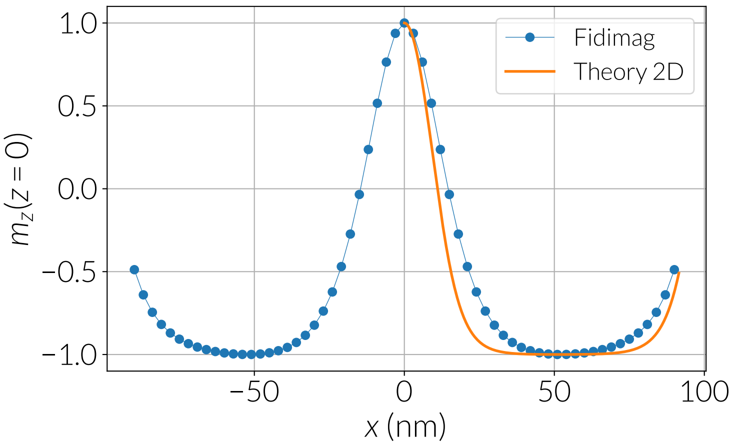


SUPP. FIG. S3. Out-of-plane component of the magnetization of a skyrmion in a cylinder ($z = 0$), as specified in Section VIsection*.8 of the main study. The profile is taken from the middle slice of the sample at $z = 0$. A comparison is performed between this profile, which was obtained using Fidimag simulations, and the two-dimensional analytical model for a skyrmion in a disk.

## S5. THREE-DIMENSIONAL PROBLEM. CODES COMPARISON

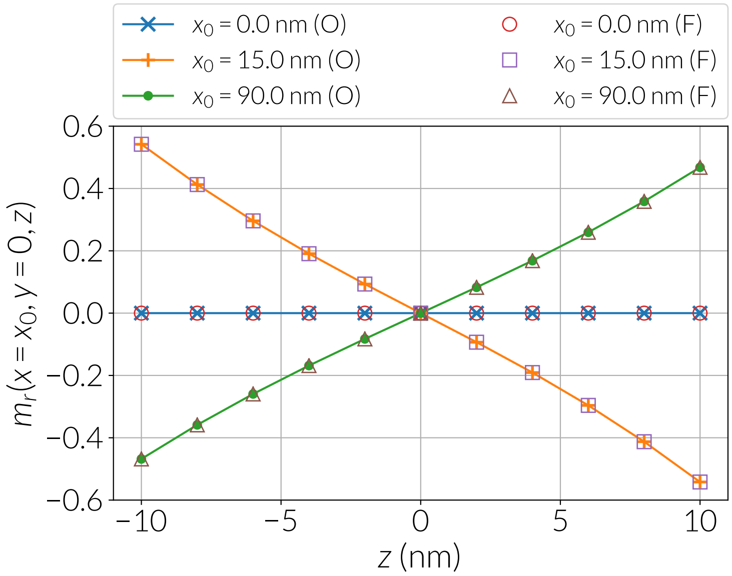


SUPP. FIG. S4. Radial component of the magnetization across the cylinder thickness at three different $(x, y)$ positions, as shown in Section VIsection*.8 of the main manuscript. This plot shows a comparison between OOMMF (O) simulations and Fidimag (F) simulations.

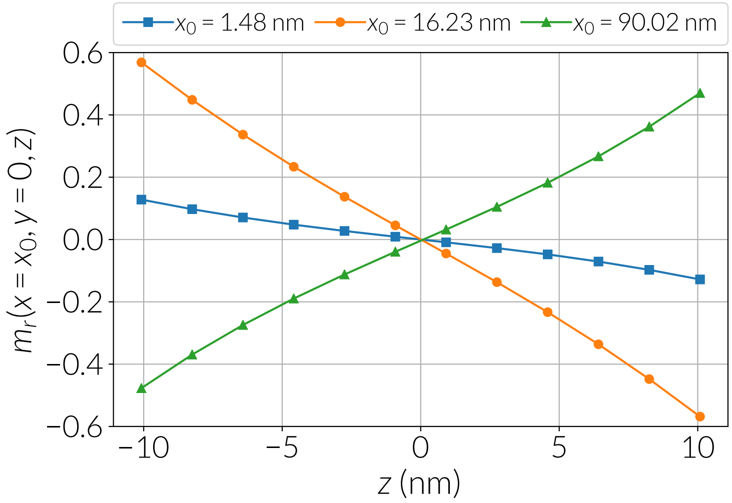


SUPP. FIG. S5. Radial component of the magnetization across the cylinder thickness at three different $(x, y)$ positions, as shown in Section VIsection*.8 of the main manuscript. This plot shows the result of MuMax3 simulations of the three-dimensional cylinder system.

| | |
|---|---|
| Block with PBCs | |
| Dimensions | $180\,\mathrm{nm} \times 180\,\mathrm{nm} \times 20\,\mathrm{nm}$ |
| Magnetic parameters | |
| $A$ | $8.78\,\mathrm{pJ\ m^{-1}}$ |
| $D$ | $1.58\,\mathrm{mJ\ m^{-2}}$ |
| $M_\mathrm{s}$ | $0.384\,\mathrm{MA\ m^{-1}}$ |
| $\mu_0\mathbf{H}$ | $(0.0, 0.4, 0.0)\,\mathrm{T}$ |

## S6. THREE-DIMENSIONAL CASE: CUBOID WITH PERIODIC BOUNDARIES

An alternative problem to the cylinder system defined in Section VIsection*.8 of the main study is a cuboid with periodic boundary conditions (PBCs). The periodicity helps to avoid the effects from the Dzyaloshinskii-Moriya interaction at the boundaries, which induce a slightly tilt of the boundary spins.

We define an isolated skyrmion in a FeGe cuboid of dimensions $180 \times 180 \times 20\,\mathrm{nm}^3$ with PBCs. We relax the system with an initial state that can be either a Bloch skyrmion profile across the sample thickness or a cylindrical region at the centre of the cuboid pointing opposite to the field and surrounded by spins in the field direction. By applying a magnetic field of $B_z = 0.4\,\mathrm{T}$, we stabilise a skyrmion tube modulated along the thickness of the system, which we choose as the $z$-direction. This skyrmion has a radius of $r_\mathrm{sk} \approx 16.1\,\mathrm{nm}$ at $z = 0$ and a radius of $r_\mathrm{sk} \approx 15.7\,\mathrm{nm}$ at the cuboid surfaces normal to $z$. As in the cylinder system of the main study, Fig. S6 exhibits similar results, but without the effects at the boundary, thus azimuthal and radial modulations of the magnetization tend to zero towards the periodic boundary of the cuboid.

In Fig. S7 we plot the linear dependence of the radial component $m_r$ as a function of $z$ at three different $(x, y = 0)$ positions in every layer: the centre, close to the skyrmion radius and at the sample boundary. We notice that the radial increment is maximal close to the skyrmion radius and it goes to zero at the centre and at the cuboid boundary.

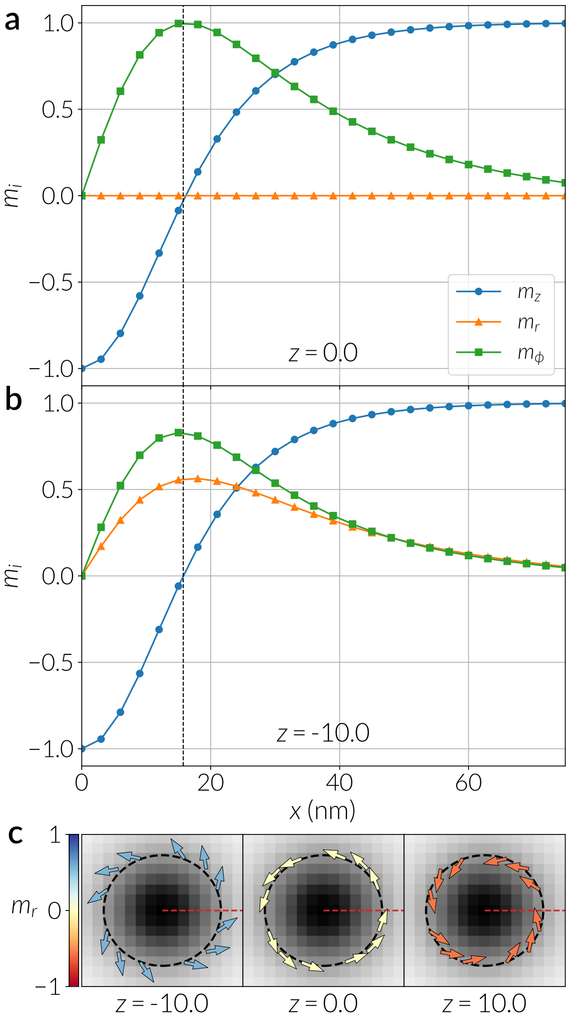


SUPP. FIG. S6. Cylindrical components of the magnetization field of an isolated skyrmion in a FeGe cuboid with periodic boundary conditions. These numerical results were obtained using the Fidimag code. (a) Profiles across the centre of an $x - y$ plane-cut of the cuboid (see red dashed line in snapshots of plot (c)) at $z = 0\,\mathrm{nm}$, which is the middle of the sample across the thickness. (b) Profiles at the bottom surface of the cuboid, which is the plane-cut at $z = -10\,\mathrm{nm}$. (c) Snapshots of the magnetization profile at (from left to right) the bottom, middle and top layers of the cuboid (which are plane-cuts) in the $z$-direction. The sample is zoomed at the central region of the layers $[(x, y) \in [-22, 22]\,\mathrm{nm} \times [-22, 22]\,\mathrm{nm}]$ where the skyrmion centre is located. Spins are drawn in a circle defined by the skyrmion radius, which is denoted by a dashed line, and are colored according to their radial component. The background illustrates the out of plane component of the magnetization $m_z$, where black means $m_z = 1$.

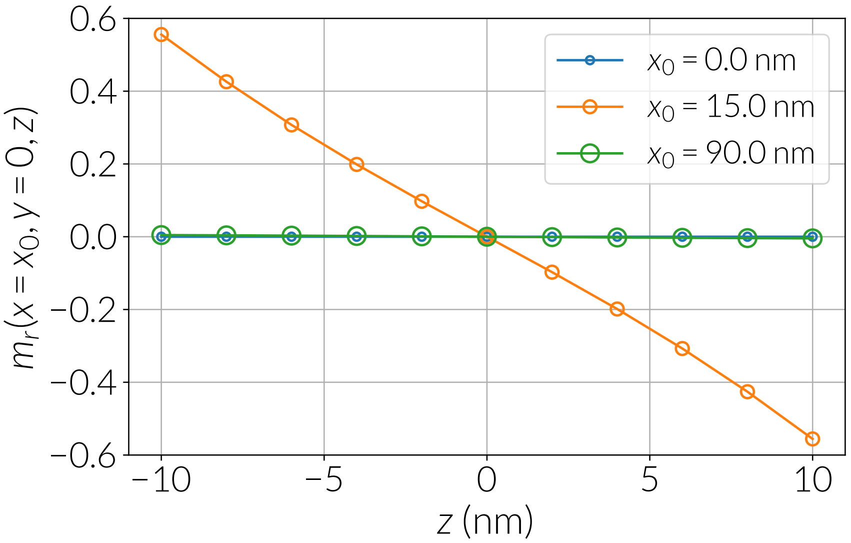


SUPP. FIG. S7. Radial component of the magnetization across the cuboid thickness at three different $(x_0, y)$ positions for every plane cut in the $z$-direction. The $y$ position is fixed at the centre of the system at $y = 0$. The chosen $x$ coordinates are at the centre of the skyrmion $(x_0 = 0)$, close to the skyrmion radius $(x_0 = 15\,\mathrm{nm})$, which is approximately 15.75 nm, and at the cuboid periodic boundary $(x_0 = 90\,\mathrm{nm})$. Data points were obtained from Fidimag simulations.

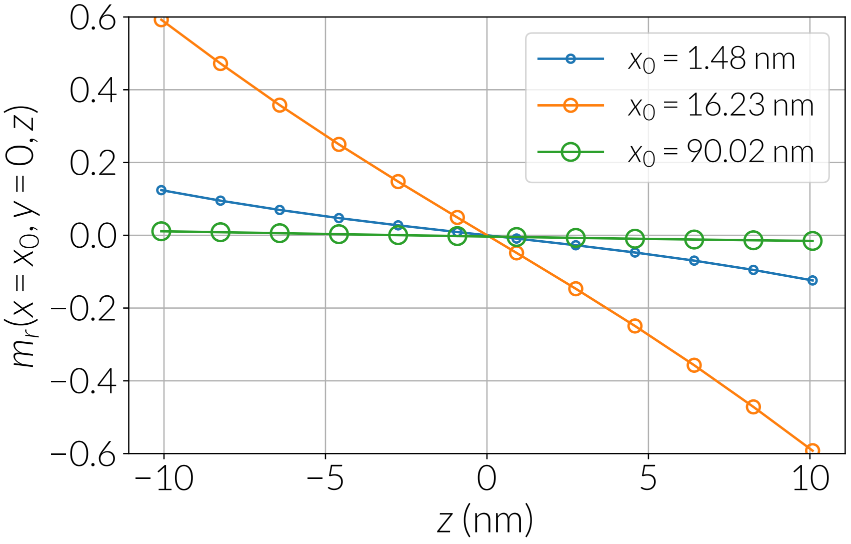


SUPP. FIG. S8. Radial component across the sample thickness (see Fig S7) obtained with MuMax3.

## S7. SPIN WAVES: RESULTS FROM OTHER CODES

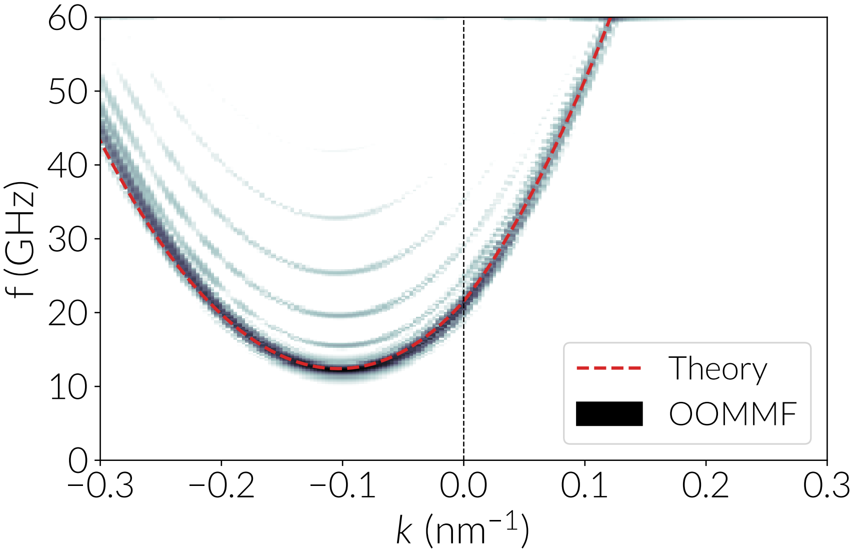


SUPP. FIG. S9. Spin wave spectrum of Damon-Eshbach spin waves obtained with the OOMMF code. The system is defined in the Dynamics problem of the main manuscript (Section VIIsection*.9).

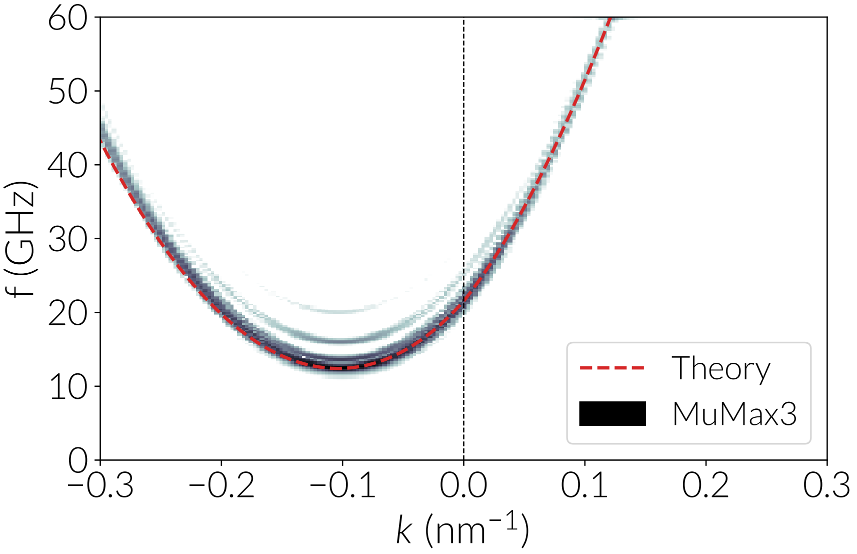


SUPP. FIG. S10. Spin wave spectrum of Damon-Eshbach spin waves obtained with the MuMax3 code. The system is defined in the Dynamics problem of the main manuscript (Section VIIsection*.9).

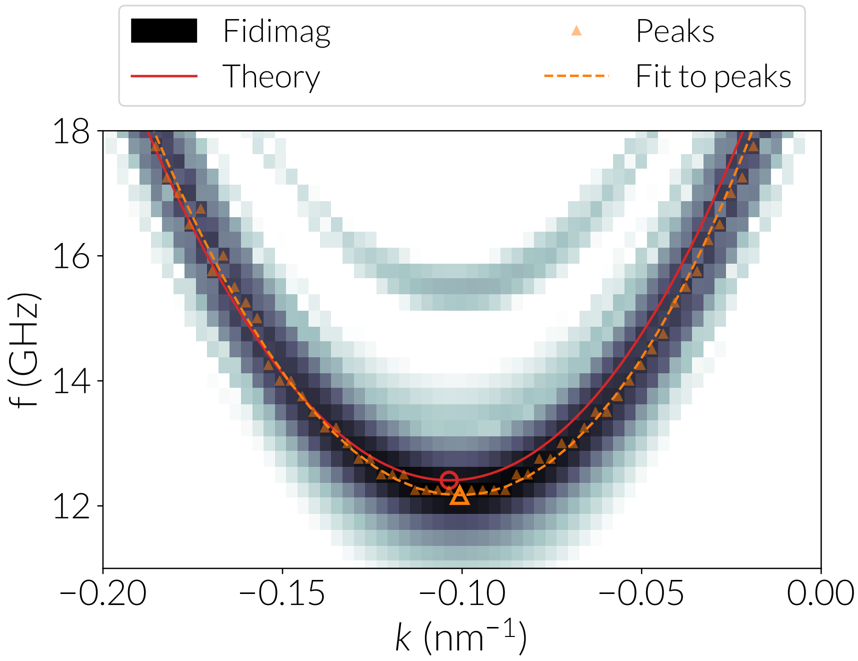


SUPP. FIG. S11. This figure shows the spin wave spectrum around the spectrum minimum, where data from Fidimag simulations is compared with the theory. The dispersion relation from the theory of Moon *et al.* [7] is shown as a continuum curve, with a circle indicating the minimum. The intensity map is the result of the simulations and is shown in logarithmic scale. The peaks of this intensity map are shown as faded triangles. A fourth order polynomial fit to the data from the peaks is shown as a dashed curve, and its minimum is indicated as an open triangle.

## S8. FINITE ELEMENT CALCULATIONS

We show here simulations performed with our finite element code Finmag.

### A. One-dimensional case

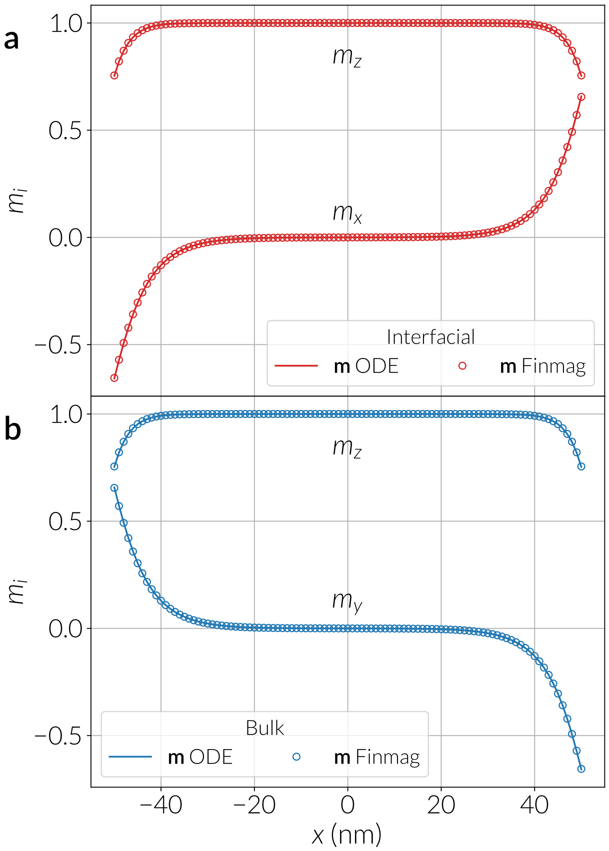


SUPP. FIG. S12. Simulations of the one-dimensional permalloy-like system using finite elements. Results are computed for a system with interfacial DMI (a) and bulk DMI (b). Simulations are compared with the semi-analytical solution of the ordinary differential equation (ODE) that describes the system, as specified in Section IVsection*.6 of the main study.

### B. Three-dimensional case

Results from finite element simulations of a skyrmion in a FeGe cylinder (this system is discussed in Section VIsection*.8 of the main text) are shown in Fig. S13, where we show the cylindrical components at the bottom and middle slices of the cylinder. Using a finite element code it is obtained a better approximation of the curved boundary of the cylinder. From these simulations we computed a skyrmion radius of 15.45 nm at a slice at the middle of the cylinder and a skyrmion radius of 15.16 nm at its top and bottom surfaces. The value of the skyrmion radius and its small variation of about 0.3 nm at the cylinder caps, is in agreement with the results of finite difference calculations, where the skyrmion has a radius of 14.91 nm at the middle slice.

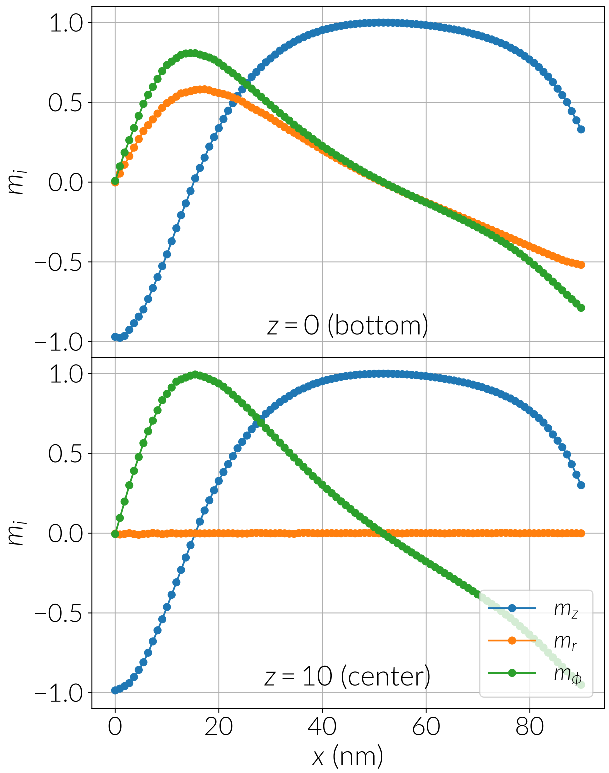


SUPP. FIG. S13. Simulation results of a skyrmion in an FeGe cylinder using our finite element code. The plot shows the cylindrical components of the magnetisation for the spins along a radius in two slices of the cylinder, as shown in Fig. 3Cylindrical components of the magnetization field of an isolated skyrmion in a FeGe cuboid with periodic boundary conditions. These numerical results were obtained using the Fidimag code. (a) Profiles across the centre of an $x - y$ plane-cut of the cuboid (see red dashed line in snapshots of plot (c)) at $z = 0\,\text{nm}$, which is the middle of the sample across the thickness. (b) Profiles at the bottom surface of the cuboid, which is the plane-cut at $z = -10\,\text{nm}$. (c) Snapshots of the magnetization profile at (from left to right) the bottom, middle and top layers of the cuboid (which are plane-cuts) in the $z$-direction. The sample is zoomed at the central region of the layers ($(x, y) \in [-22, 22]\,\text{nm} \times [-22, 22]\,\text{nm}$) where the skyrmion centre is located. Spins are drawn in a circle defined by the skyrmion radius, which is denoted by a dashed line, and are colored according to their radial component. The background illustrates the out of plane component of the magnetization $m_z$, where black means $m_z = 1$figure.3 of the main study. These slices are the bottom cylinder cap and a slice at the centre of the cylinder.

We performed an additional test to the finite-element results by comparing the Finmag calculations with the non-publicly available code by R. Hertel, which is a successor of the TetraMag code [8, 9]. In Fig. S14 it can be observed a good agreement between both simulation packages.

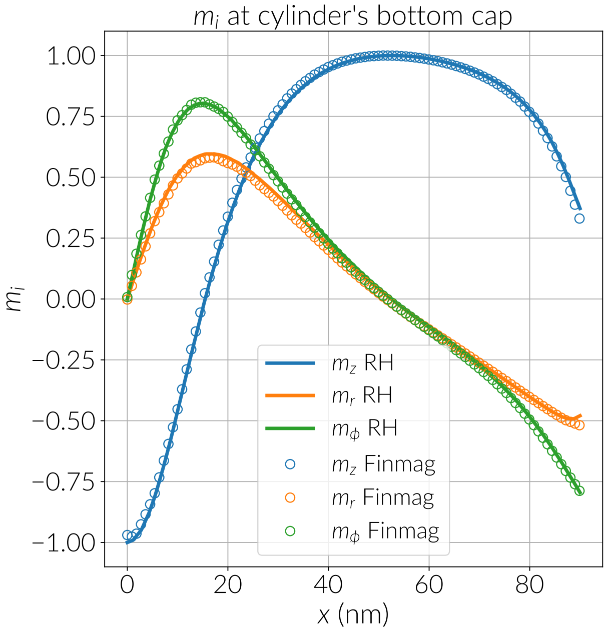


SUPP. FIG. S14. Comparison of the cylindrical components in the cylinder system between Finmag and R. Hertel's (RH) finite-element code simulations. The components were extracted at the bottom surface of the cylinder.

[1] Yosida, K. *Theory of Magnetism*, vol. 122 of *Springer Ser. Solid-State Sci.* (Springer-Verlag Berlin Heidelberg, 1996), 1 edn.

[2] Dzyaloshinskii, I. A thermodynamic theory of "weak" ferromagnetism of antiferromagnetics. *J. Phys. Chem. Solids* **4**, 241–255 (1958).

[3] Dzyaloshinskii, I. E. Theory of helicoidal structures in antiferromagnets. II. Metals. *Soviet Physics JETP* **19**, 960–971 (1964).

[4] Moriya, T. Anisotropic superexchange interaction and weak ferromagnetism. *Phys. Rev.* **120**, 91–98 (1960).

[5] Landau, L. D. & Lifshitz, E. *Statistical Physics*, vol. 5 of *Course of Theoretical Physics* (Butterworth-Heinemann, 1980), third edn.

[6] Leliaert, J. *et al.* Fast micromagnetic simulations on GPU-recent advances made with mumax 3. *J. Phys. D: Appl. Phys.* (2018).

[7] Moon, J. J. H. *et al.* Spin-wave propagation in the presence of interfacial Dzyaloshinskii-Moriya interaction. *Phys. Rev. B* **88**, 1–6 (2013).

[8] Hertel, R. Guided Spin Waves. In *Handbook of Magnetism and Advanced Magnetic Materials*, 1003–1020 (John Wiley & Sons, 2007).

[9] Kakay, A., Westphal, E. & Hertel, R. Speedup of FEM micromagnetic simulations with graphical processing units. *IEEE Trans. Magn.* **46**, 2303–2306 (2010).
